# Supplementary material for: Odd Droplets: Fluids with Odd Viscosity and Highly Deformable Interfaces
Source: arXiv:2503.21649 source file (2025-03-27)

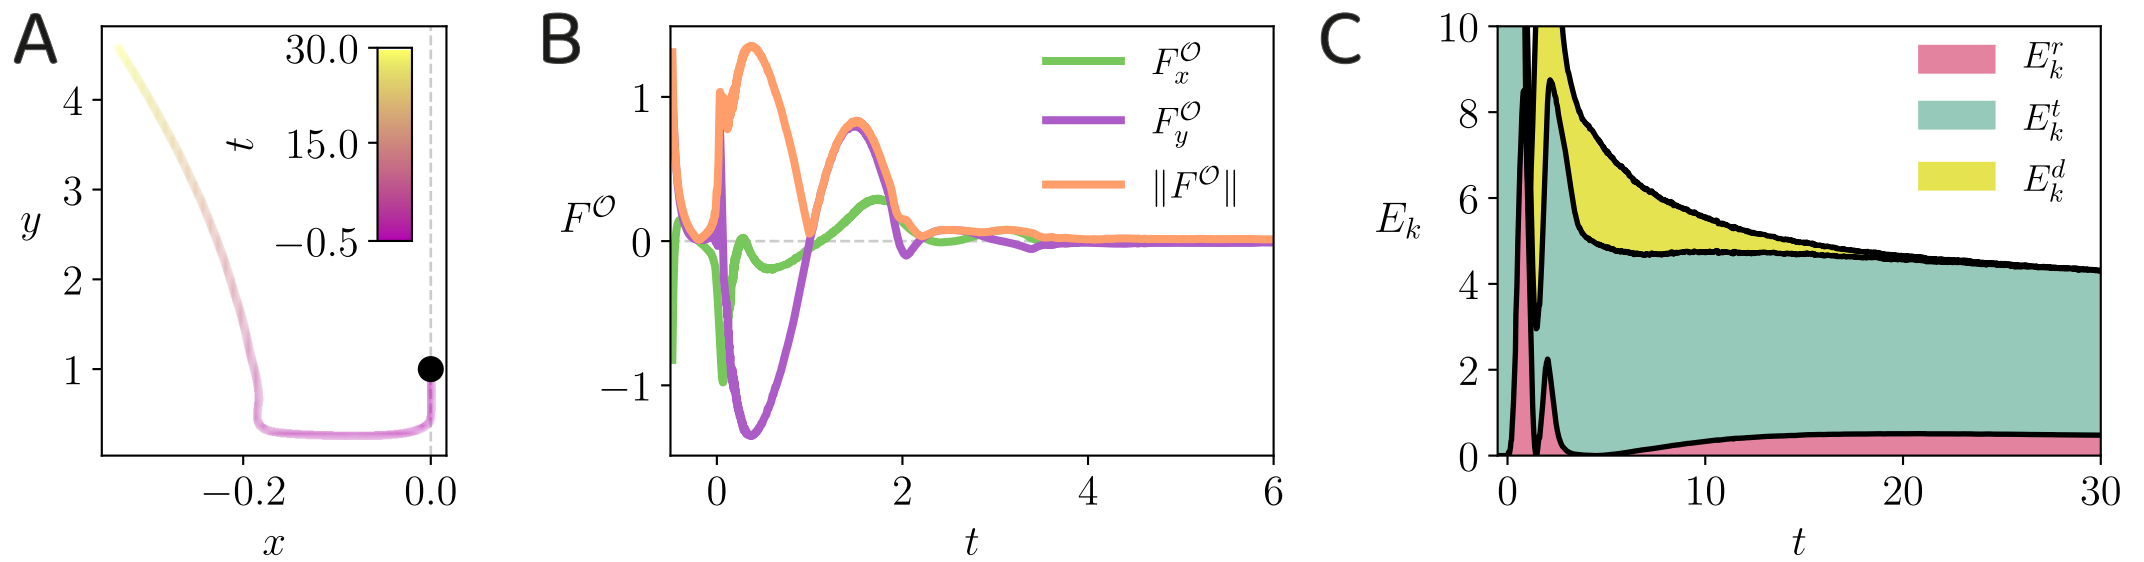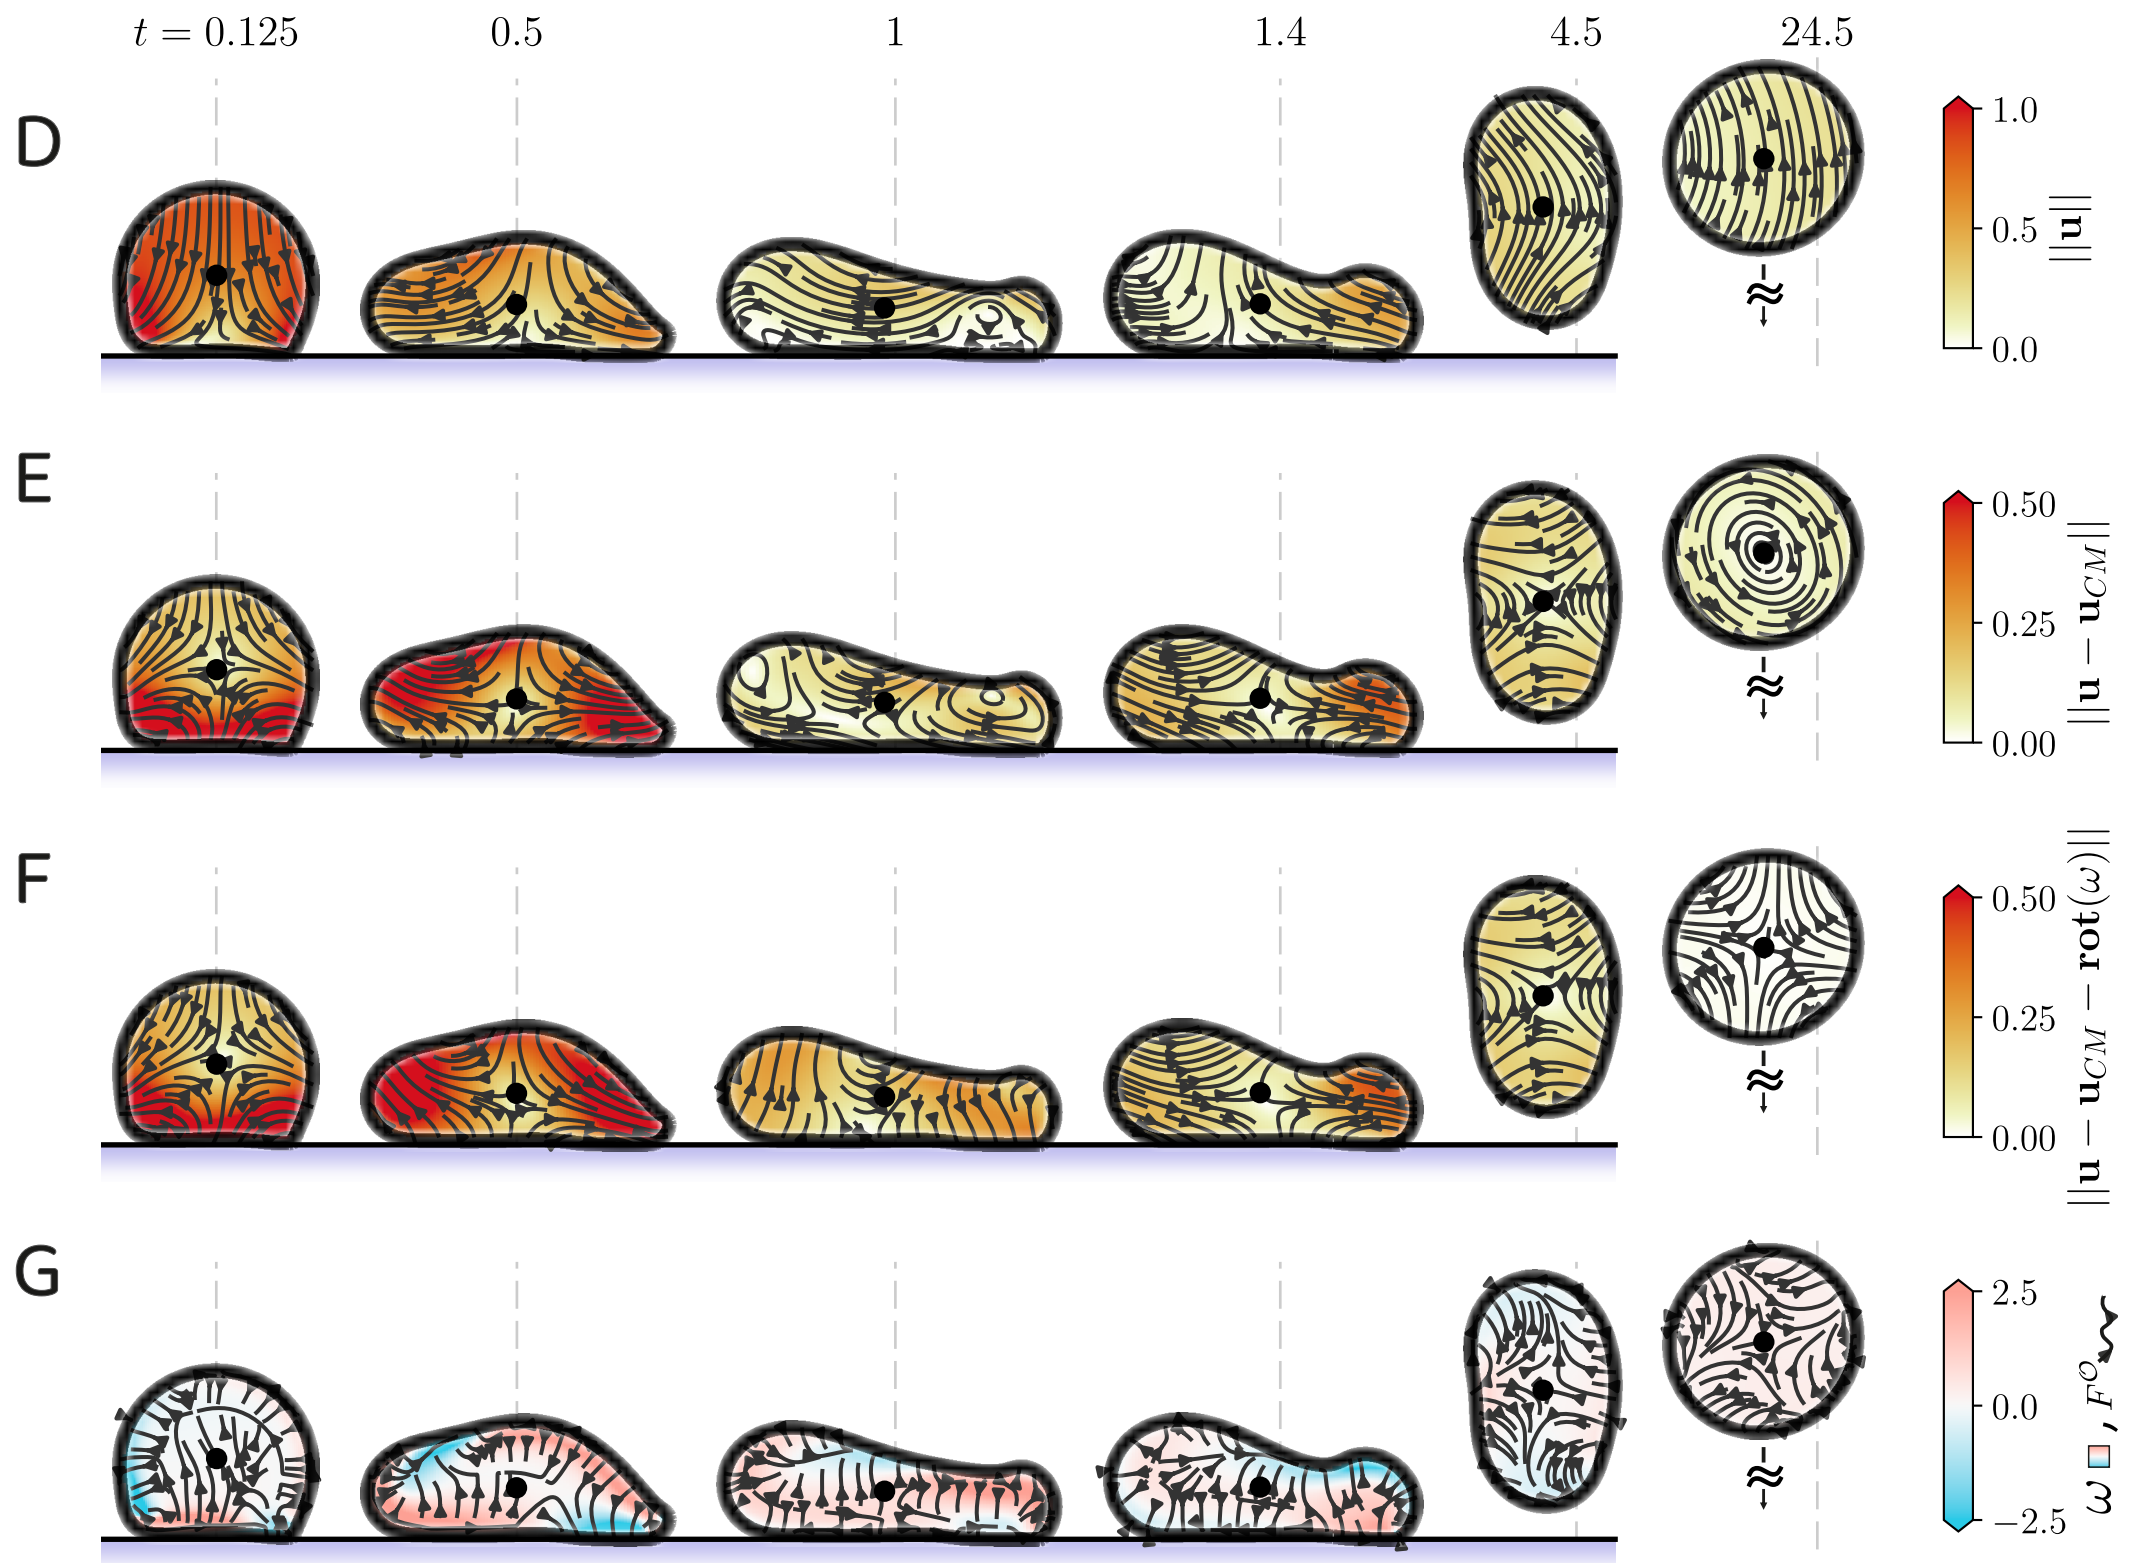

Supplement: Supplementary file 1 [file fig_appendix_fields_case1.pdf]
