# Supplementary material for: Odd Droplets: Fluids with Odd Viscosity and Highly Deformable Interfaces
Source: arXiv:2503.21649 source file (2025-03-27)

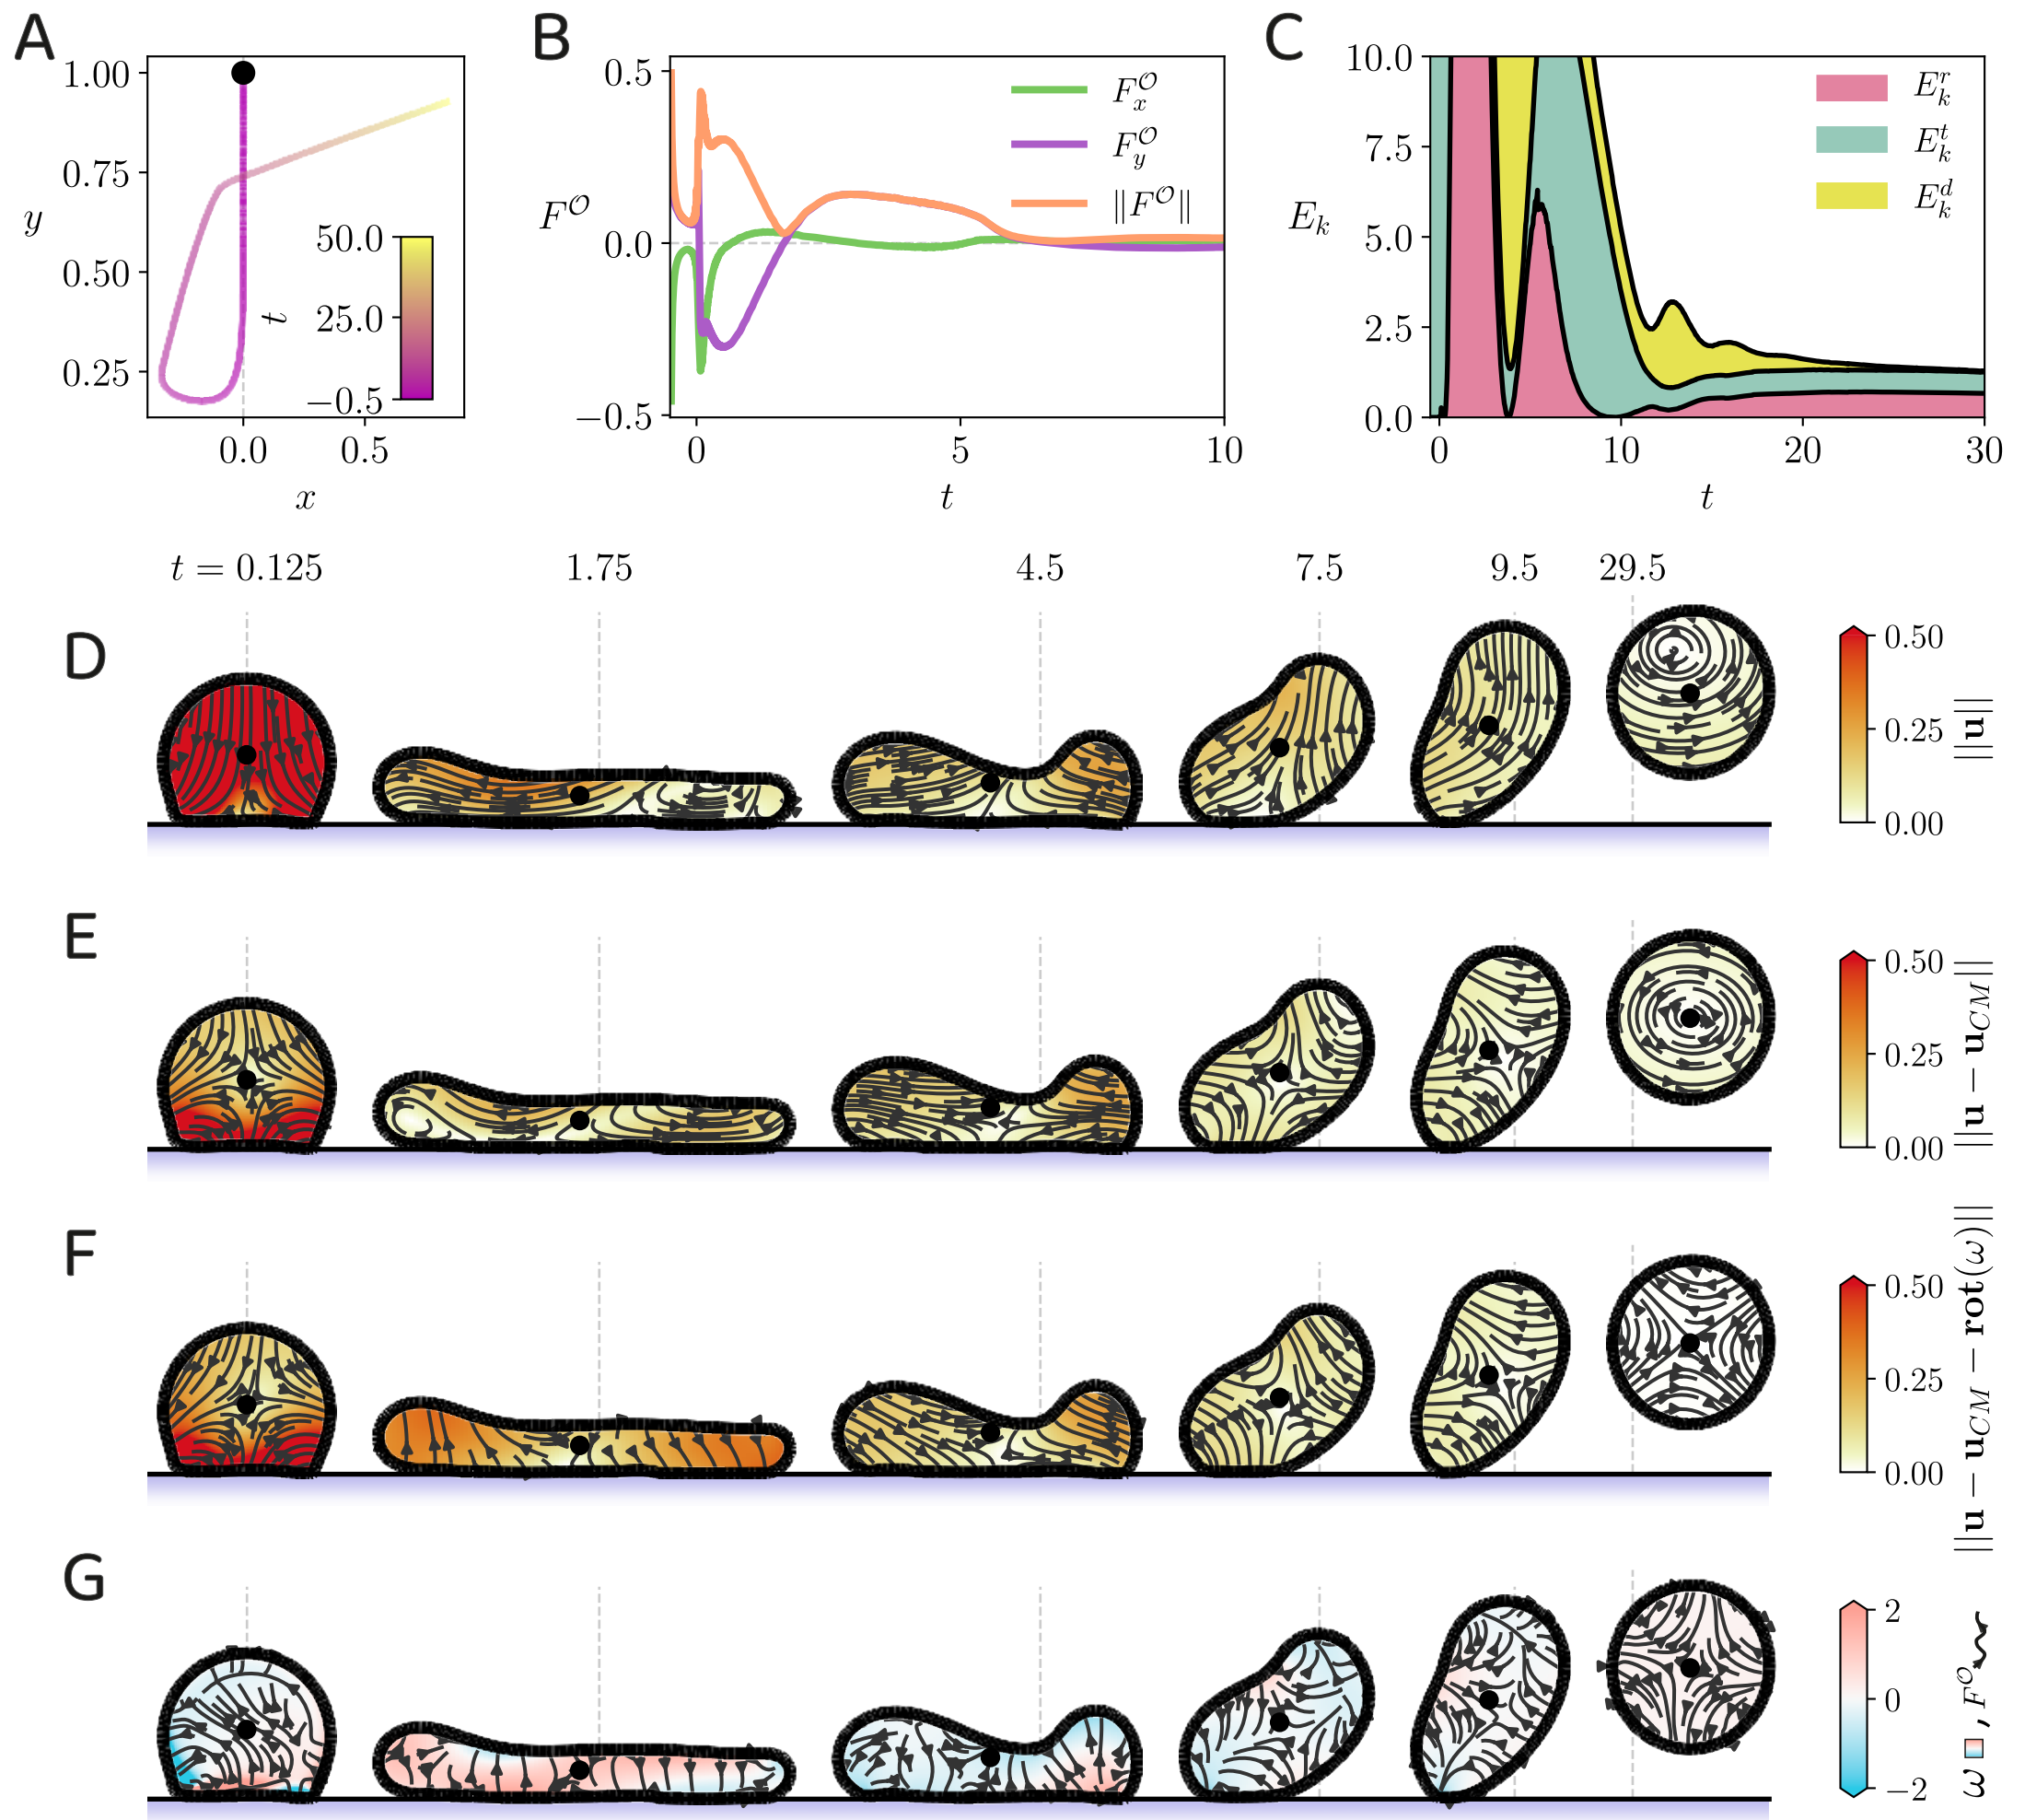

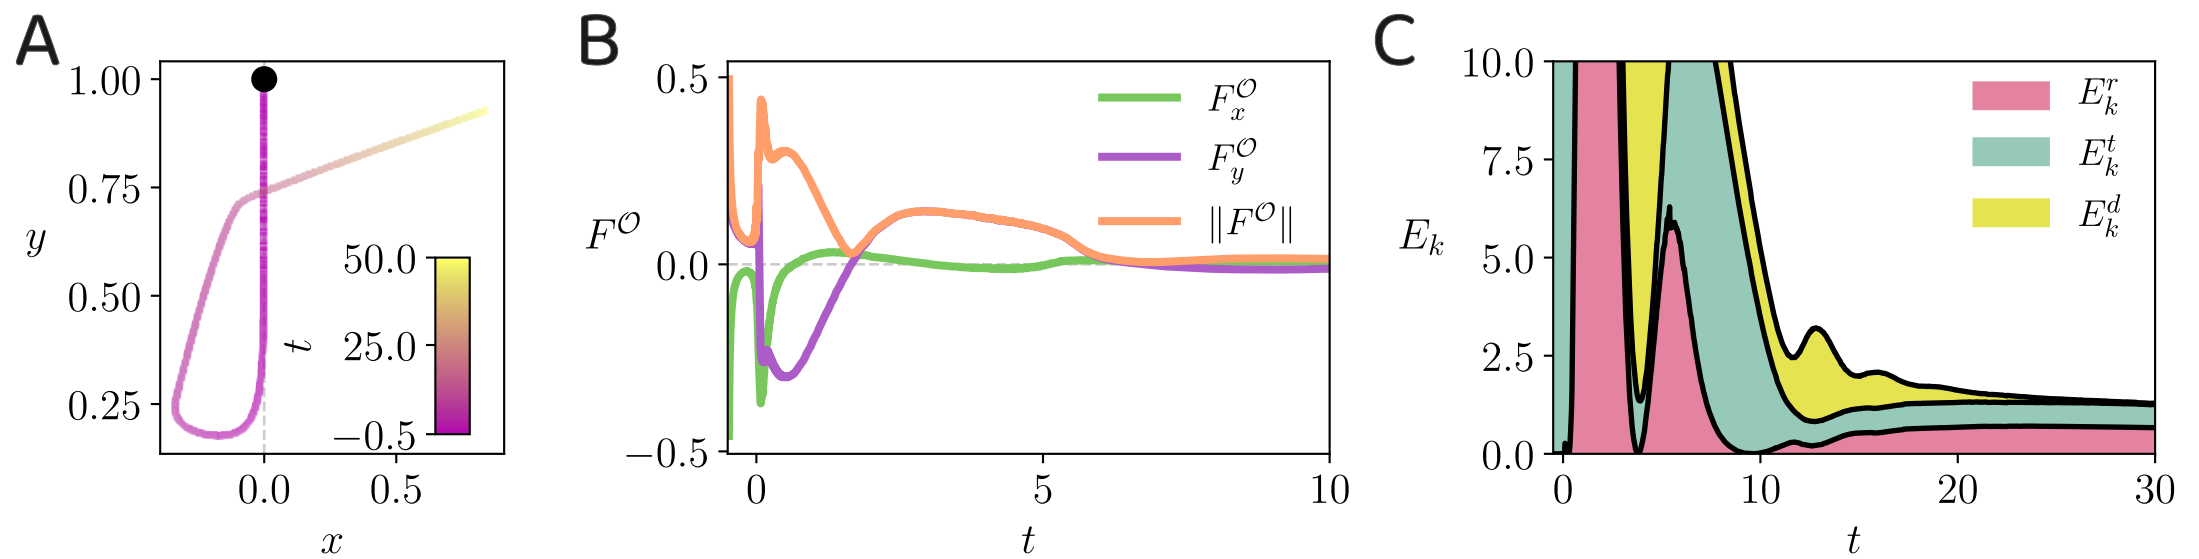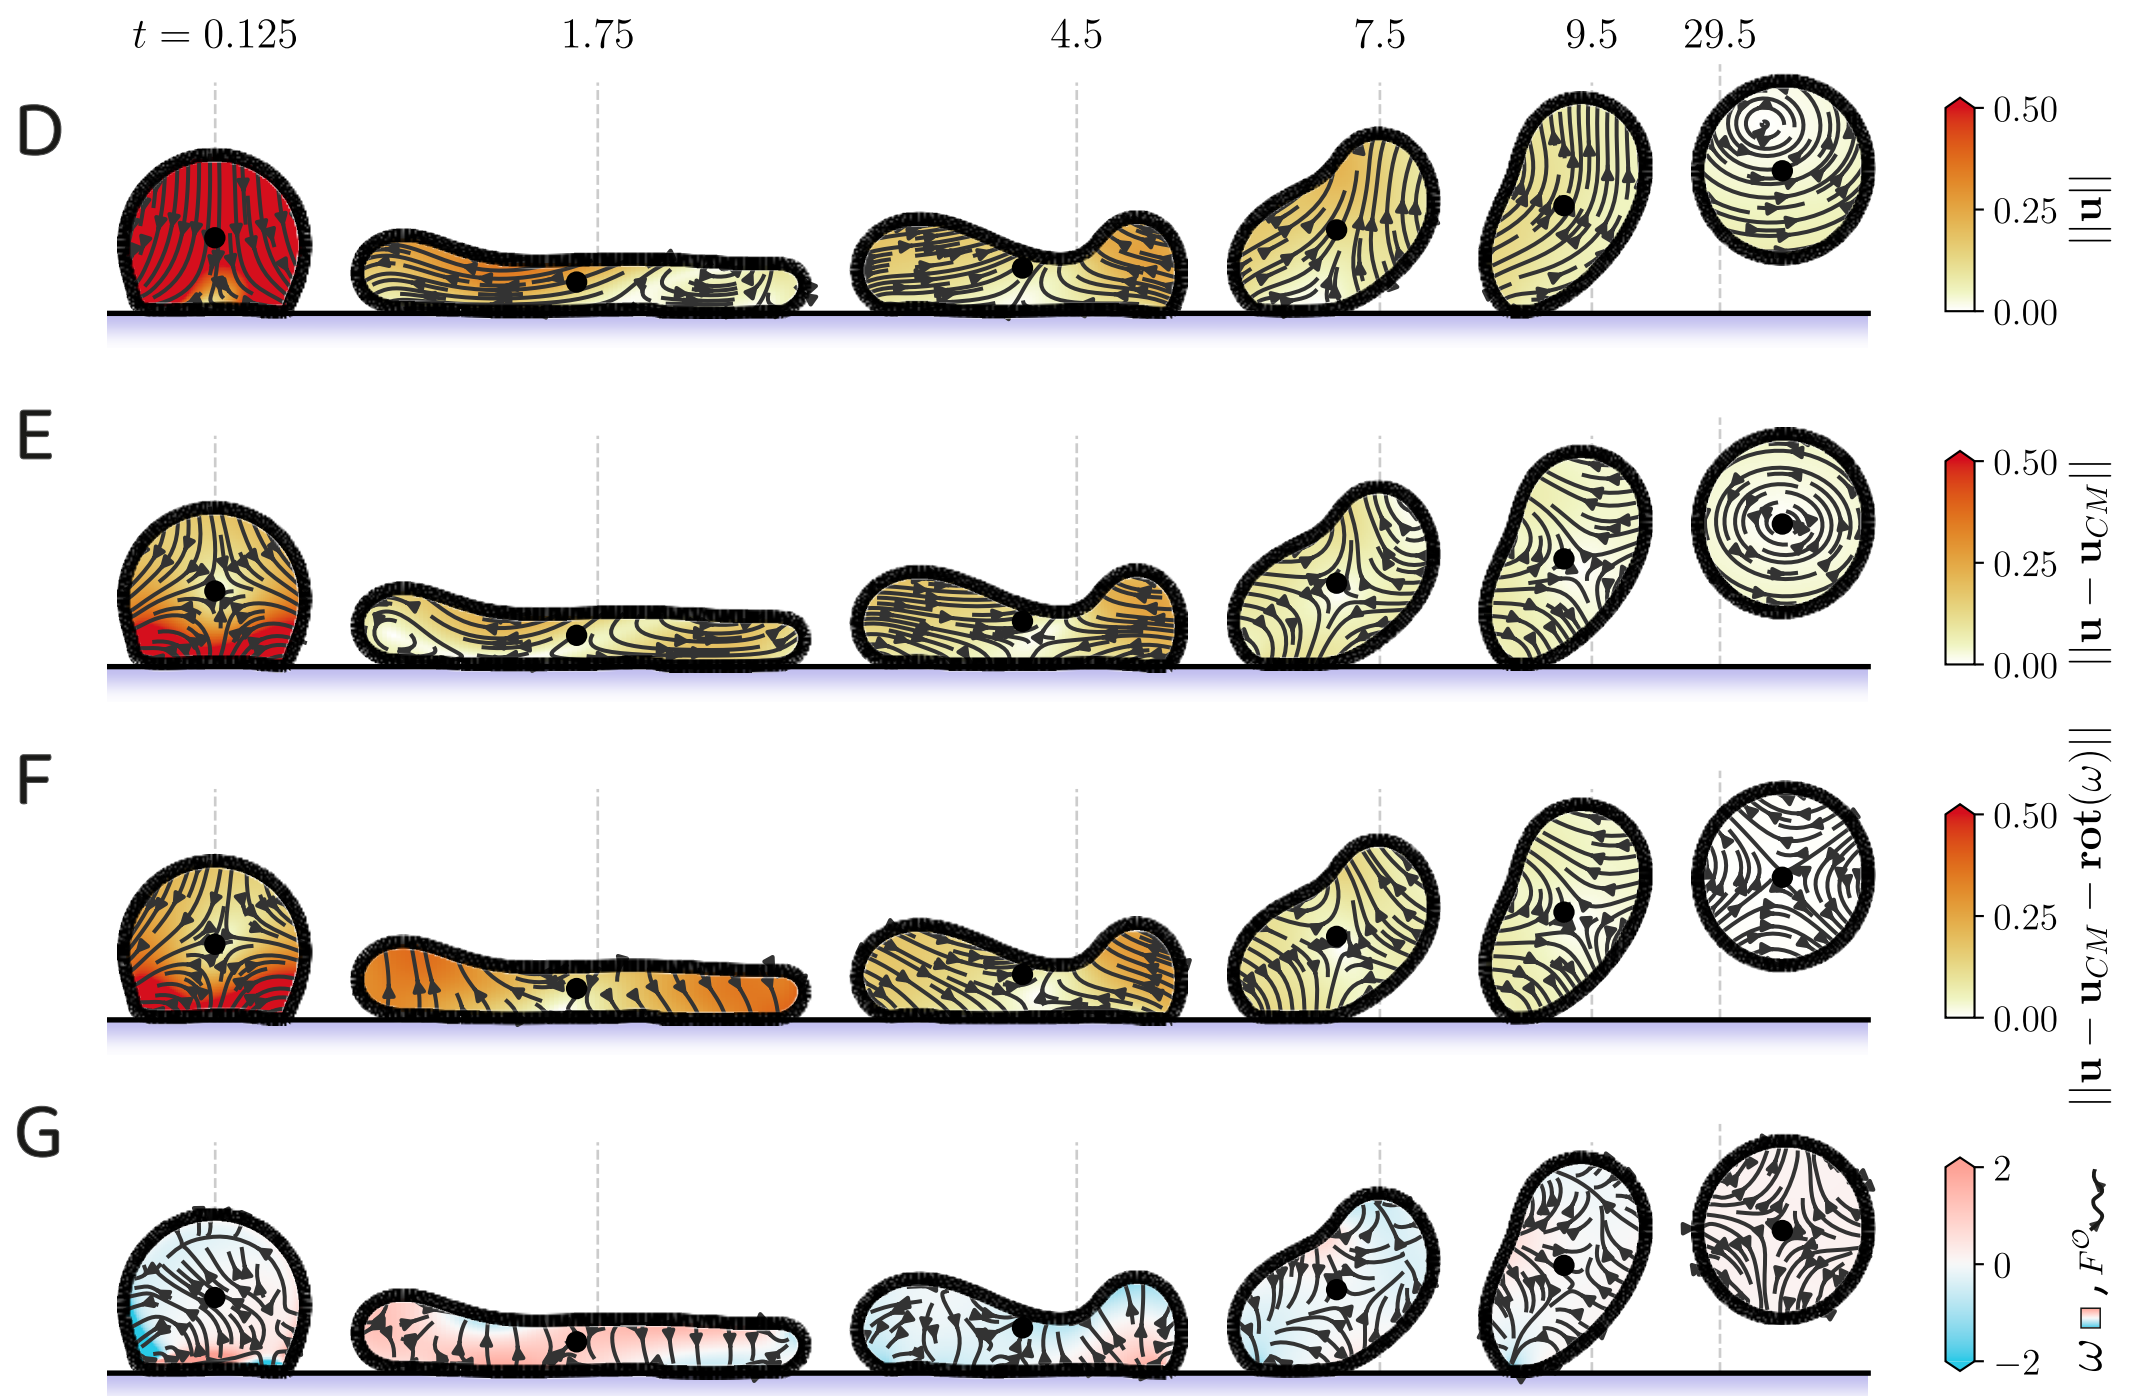

Supplement: Supplementary file 2 [file fig_appendix_fields_case2.pdf]
